# Supplementary material for: MAVEN: Multi-Agent Variational Exploration
Source: arXiv:1910.07483 source file (2020-01-20)
Supplement: Supplementary file 1 [file defs.tex]

\section{Definitions}

\subsection{Auxiliary definitions}
\label{app:NMF}

\begin{definition}
	A binary relation $\mathcal{R}$ on a set $\mathcal{S}$ is given by $\mathcal{R} \subseteq \mathcal{S}\times\mathcal{S}$ 
\end{definition}

\begin{definition}
	$\mathcal{R}$ is symmetric if $\mathcal{R}(a,b)\implies \mathcal{R}(b,a)$
\end{definition}

\begin{definition}
	$\mathcal{R}$ is reflexive if $\mathcal{R}(a,a), \forall a\in \mathcal{S}$
\end{definition}

\begin{definition}
	$\mathcal{R}$ is transitive if $\mathcal{R}(a,b) \land \mathcal{R}(b,c) \implies \mathcal{R}(a,c)$
\end{definition}

\begin{definition}
	$\mathcal{R}$ is equivalence if its reflexive, symmetric and transitive.
\end{definition}

\begin{definition}
	$\mathcal{R}$ is a total order if $\forall a,b \in \mathcal{S}, \mathcal{R}(a,b) \lor \mathcal{R}(b,a)$ but not both. 
\end{definition}

\begin{definition}
	If $\mathcal{R}$ is an equivalence relation then it can be partitioned into equivalence classes with $\mathcal{P}(\mathcal{R},\mathcal{S})\triangleq \{\mathcal{C}_i\}$, where $\mathcal{C}_i \subseteq \mathcal{S}, \forall a,b \in \mathcal{C}_i\implies\mathcal{R}(a,b)$ and $ \mathcal{C}_i \cap  \mathcal{C}_j$ is empty if $i\neq j$.
\end{definition}

\begin{definition}
For partitions $\mathcal{P}_1,\mathcal{P}_2$, $\mathcal{P}_1$ is a filtrate of $\mathcal{P}_2$ if $\forall \mathcal{C}_i \in \mathcal{P}_2, \exists \mathcal{D}_j \in \mathcal{P}_1$ s.t. $\mathcal{C}_i = \cup_j \mathcal{D}_j$  
\end{definition}

\begin{definition}
$\mathcal{F}(\mathcal{P}_1,\mathcal{P}_2)$	is the common filtrate of $\mathcal{P}_1,\mathcal{P}_2$ if it is a filtrate of both.
\end{definition}

\begin{definition}
	$\mathcal{G}(\mathcal{P}_1,\mathcal{P}_2)$	is the greatest common filtrate of $\mathcal{P}_1,\mathcal{P}_2$ if $\forall$ common filtrates $ \mathcal{F}(\mathcal{P}_1,\mathcal{P}_2), |\mathcal{F}|\geq|\mathcal{G}|$ where $|\cdot|$ denotes set size.
\end{definition}
